# Supplementary material for: 2D abrupt nano-junctions blending sp-sp2 bonds on atomically precise heterostructures
Source: arXiv:2601.19437 source file (2026-03-25)
Supplement: Supplementary file 1 [file SI-test.pdf]

# Supporting Information: Graphene Nanoribbon - Graphdiyne Lateral Heterojunctions with Atomically Abrupt Interfaces

Alice Cartoceti[1†], Simona Achilli[2,3†], Masoumeh Alihosseini[2], Adriana E. Candia[4], Enrico Beltrami[2], Paolo D'Agosta[1], Alessio Orbelli Biroli[5], Francesco Sedona[6], Andrea Li Bassi[1], Jorge Lobo Checa[7,8], Carlo S. Casari[1]

[1*]Department of Energy, Politecnico di Milano, via Lambruschini 6, Milano, 20156, Italy.
[2]Department of Physics 'Aldo Pontremoli', Università degli Studi di Milano, Via G. Celoria 16, Milano, 20133, Italy.
[3]INFN Sezione di Milano and 'European Theoretical Spectroscopy Facility' (ETSF), Via G. Celoria 16, Milano, 20133, Italy.
[4]Instituto de Física del Litoral, Consejo Nacional de Investigaciones Científicas y Técnicas, Universidad Nacional del Litoral (IFIS-Litoral, CONICET-UNL), Santa Fe, 3000, Argentina.
[5]Department of Chemistry, Università di Pavia, Via Taramelli 12, Pavia, 27100, Italy.
[6]Dipartimento di Scienze Chimiche, Università Degli Studi Di Padova, Padova, 35131, Italy.
[7]Instituto de Nanociencia y Materiales de Aragon (INMA), CSIC-Universidad de Zaragoza, Zaragoza, 50009, Spain.
[8]Departamento de Física de la Materia Condensada, Universidad de Zaragoza, Zaragoza, 50009, Spain.

Contributing authors: alice.cartoceti@polimi.it; simona.achilli@unimi.it;
[†]These authors contributed equally to this work.

# On-surface synthesis of hGDY-aGNR heterostructure

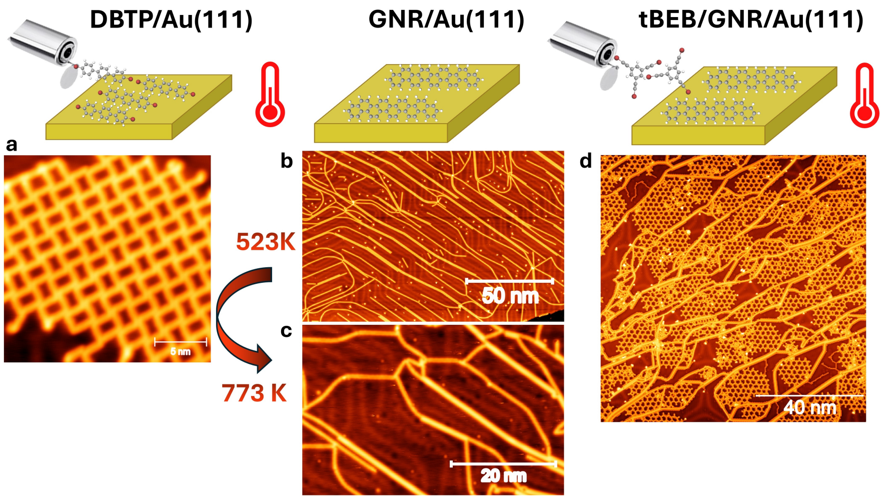


**Figure S1**: Schematic representation of the on-surface synthesis of lateral hGDY-aGNR heterostructures. For each step, a LT-STM image of the sample is reported. (a) As-deposited DBTP molecules on Au(111) at room temperature. (b) PPP chains formed upon annealing of the sample at 523 K. (c) aGNRs obtained upon annealing of the sample at 773 K. (d) Lateral heterostructures obtained upon the evaporation of tBEB molecules on aGNRs and sample annealing at 400 K. STM setpoint: (a) -0.01V/100pA, (b) 100mV/50pA, (c) 300mV/50pA, (d) -50mV/10pA.

## Polydispersity of aGNRs width

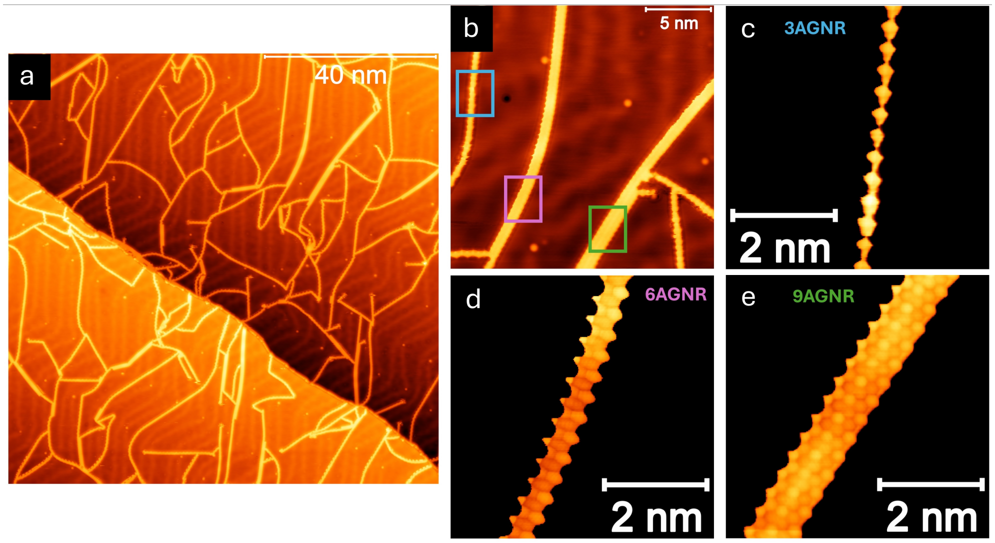


**Figure S2**: Large scale (a) and atomically resolved (b-e) LT-STM image of aGNRs on Au(111). (c-e) Close up of the squared regions in (b), namely corresponding to 3-aGNR (blue square, c), 6-aGNR (pink square, d) and 9-aGNR (green square, e). STM setpoint: (a) -20mV/100pA, (b) -10mV/130pA, (c) -2mV/60pA, (d) -2mV/60pA, (e) -2mV/60pA.

## hGDY termination and bond dissociation energy

We consider two possible terminations of the freestanding hGDY in a rectangular unit cell, namely one with only one Au atom and another one with a terminal Au-Br complex. The systems are periodic along the horizontal direction. We evaluated the stability of the two models by considering the total energy difference between a hGDY fragment terminated with Au-Br and only with Au, by including in the energy balance the contribution of the Br atoms removed. The calculated quantity also furnishes the dissociation energy of the Au-Br complex at the termination of the hGDY. We found that the Au-Br terminated case is 3.40 eV more stable than the Au-terminated hGDY, thus we can conclude that the Au dangling bonds of the hGDY have the tendency to saturate with Br atoms.

To calculate the dissociation energy of C-Au we compared the total energy of the infinite metalated hGDY with that of the Au-terminated, and we identified this difference as the energy required to break C-Au bonds, once the number of atoms in this computation has been properly considered.

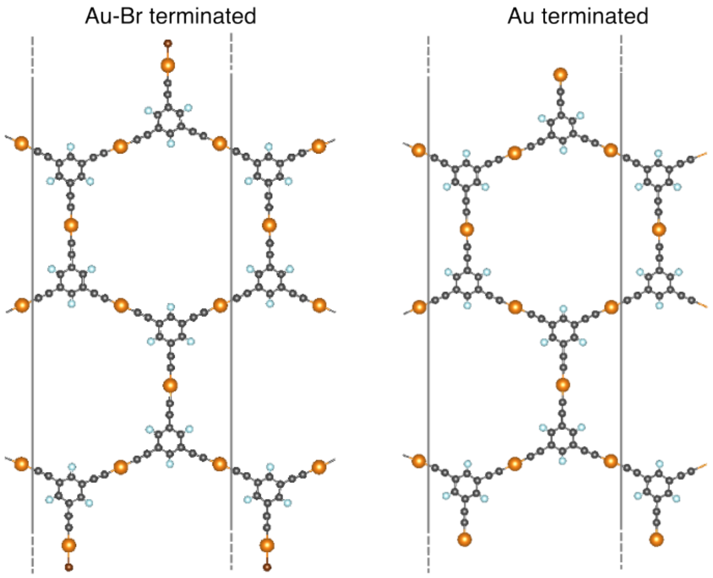


**Figure S3**: Models of hGDY terminated with Br-Au complex (left) or only Au (right). The horizontal periodicity is marked by the two vertical gray lines corresponding to segments of the unit cell edges. In the vertical direction, the two structures face a vacuum region of tens of angstroms to guarantee the decoupling between the replicas.

## A and B linking configurations between hGDY and aGNRs

The statistical prevalence of the A configuration over the B configuration can be explained by the most favorable matching of the two sublattices in the former. Indeed, in A configuration, the periodicity of the hGDY differs from the one of the aGNR of $\sim 2.2\%$, while in the B configuration this difference is of $\sim 5\%$. As a consequence the B configuration is 2.58 eV less stable than configuration A.

In both configurations, upon linking, the two subsystems rearrange leading to a compression of the aGNR along the armchair direction and an expansion of the hGDY in the horizontal direction.

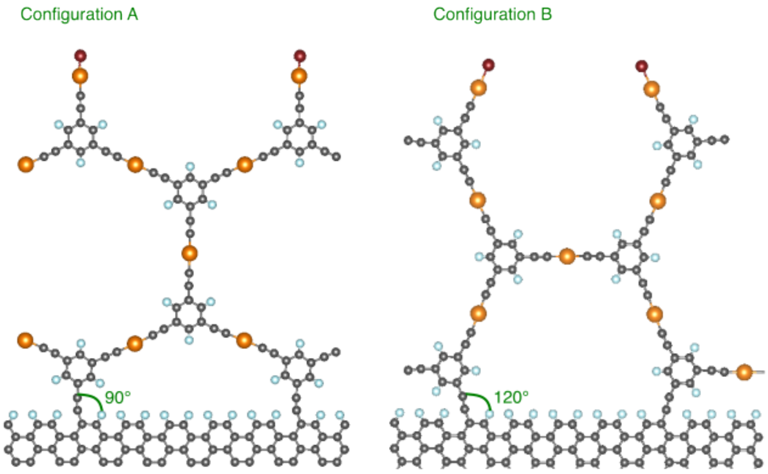


**Figure S4**: Ball-and-stick atomic model of the two possible configurations, called for simplicity "A" and "B".

## Additional STM images of the covalent bonding

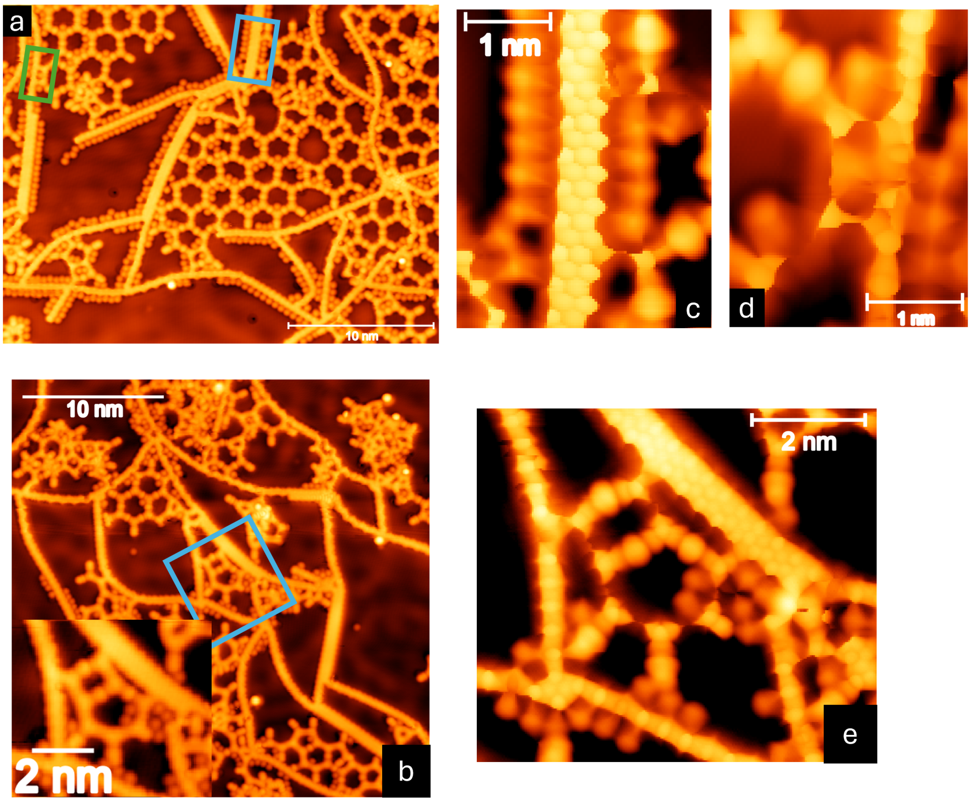


**Figure S5**: (a,b) Large-scale LT-STM image of the system upon the formation of covalent bonds between hGDY metalated network and 3- and 6-aGNRs. (b,inset) close up of the blue rectangle in (b). Br-functionalized STM tip. (c) Close up of the blue rectangle in (a). (d) Close up, flipped by 180°, of the green rectangle in (a). (e) Close up of the blue rectangle in (b). CO-functionalized STM tip. STM setpoint: (a) -10mV/80pA, (b, b inset) -30mV/80pA, (c) -10mV/80pA, (d) -3mV/80pA, (e) -2.7mV/50pA.

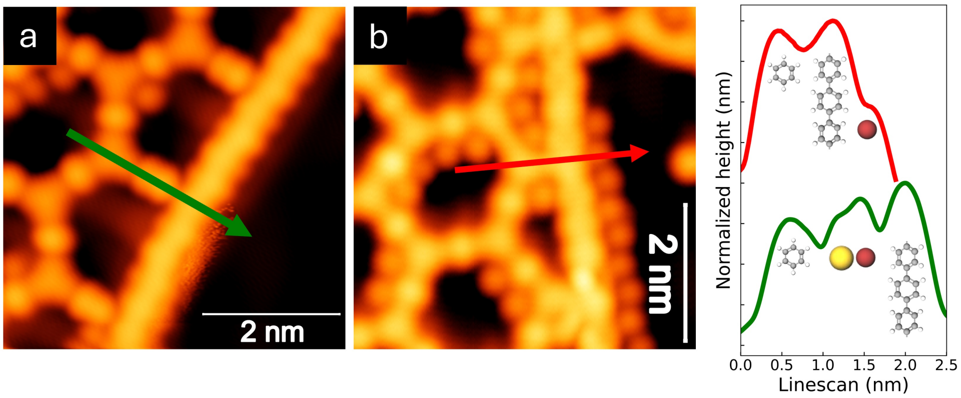


**Figure S6**: High resolution LT-STM image of the aGNR-hGDY heterostructure on Au(111) before (a) and after (b) the formation of the heterojunctions, i.e., upon annealing at 400 K and 530 K, respectively. Line profile taken along the green and red arrows on (a) and (b) are shown on the right, together with the ball-and-stick atomic model of benzene ring, gold adatom, Br atom and PPP. STM setpoint: (a) 100mV/100pA, (b) -1mV/80pA.

## Atomic hydrogen dosage

The gas pressure must be controlled very carefully in presence of sp-carbon hybridized species, since H atoms react not only with Br atoms but also with the unsaturated sp-carbon bonds and, thus, a too large hydrogen pressure determines the complete disruption of the hGDY metalated network, as can be appreciated in Figure S7, where we employed a pressure of $1 \times 10^{-7}$ mbar.

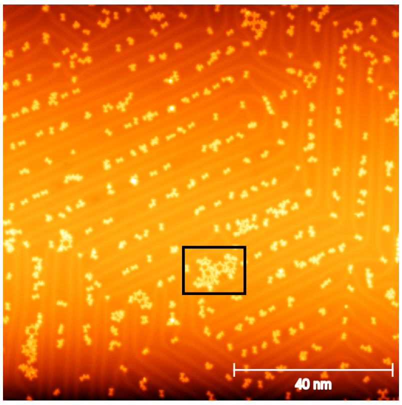


**Figure S7**: Large-scale LT-STM image of tBEB molecules on Au(111) after atomic hydrogen dosage with a pressure of $1 \times 10^{-7}$ mbar. Mainly tBEB dimers and just a small portion of extended network can be seen (black square). STM setpoint: 500mV/50pA.

With a pressure of $2 \times 10^{-8}$ mbar, we could reduce the average number of Br atoms on the surface to 0.19 $nm^{-2}$ without destroying the hGDY network, and we observed an increase in the linking efficiency with the aGNRs, as shown by the red curve in Figure S8. Also the efficiency in the transition of the hGDY from organometallic to covalent is largely influenced by the presence of Br atoms, as shown by the green curve in Figure S8.

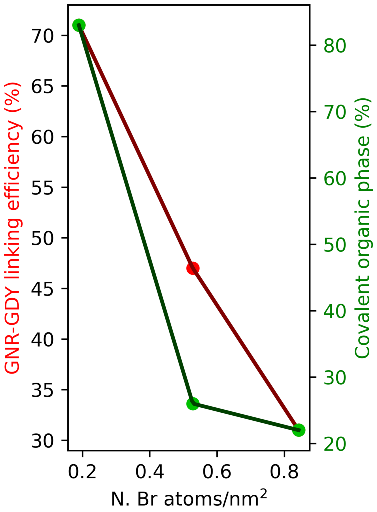


**Figure S8**: Efficiency in the formation of hGDY-aGNR covalent bonds (red curve) and percentage of covalent links within the hGDY network (green curve) as a function of the average number of Br atoms per unit area.

However, upon hydrogen dosage at $2 \times 10^{-8}$ mbar, the final system does not maintain the same degree of order as the pristine one, and some degradation effect can be observed, as shown in Fig.S9, which compares the system before and after the atomic hydrogen dosage. Such irregularity is related to the reduction of Au-coordinated regions in the hGDY, which leads to uncontrolled covalent polymeric structures.

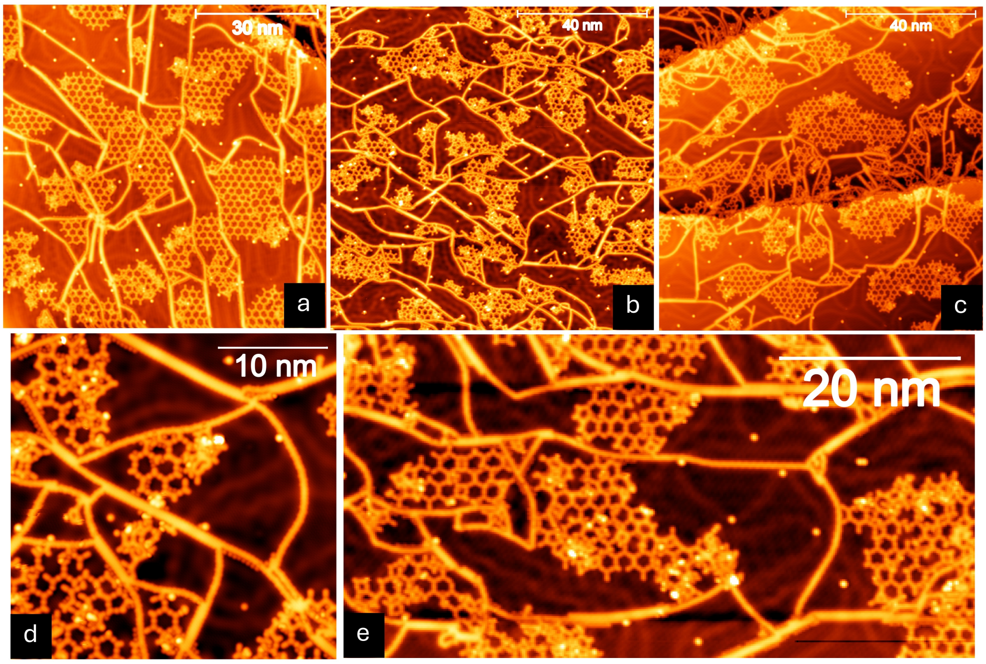


**Figure S9**: Large-scale LT-STM images of the hGDY-aGNR heterostructure after the annealing at 530 K (a) and after the consequent atomic H dosage at RT, with a pressure of $2 \times 10^{-8}$ mbar, and the following annealing at the same temperature, i.e. 530 K (b-c) (see Methods). High-resolution LT-STM images of disordered hGDY domains after H dosage (d-e). STM setpoints: (a) 300mV/50pA, (b) -81mV/80pA, (c) 500mV/50pA, (d) 100mV/50pA, (e) 100mV/50pA.

## PDOS on selected atoms in the heterostructure

In Figure S10a and b, we report the PDOS on C atoms located at the linking site ($C_1$, $C_2$, $C_3$, with labels as reported in Figure 3f of the main text) and in the central region of hGDY and aGNR. From the comparison of these data it is evident that the features at -1.8 eV, 0.1, and between 0.2 and 2.5 eV, in the green line of Figure S10a are localized states on $C_3$ atom that decay in the inner of the hGDY, as can be understood by their absence in the blue/cyan lines. The same conclusion holds for the state at the Fermi level in Figure S10b which is localized at the interface and decays in the inner of the aGNR (green line). These localized states do not contribute to electronic transport.

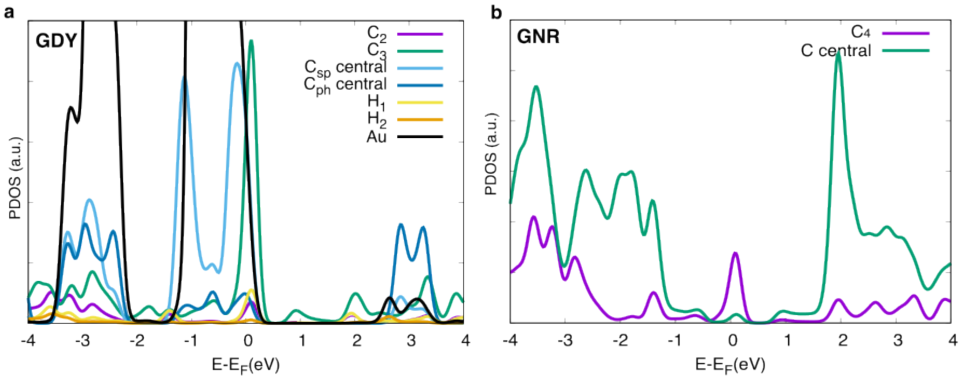


**Figure S10**: PDOS on C atoms in different position of the hGDY (a) and aGNR in the freestanding "2H" heterostructure. In a), the PDOS on H atoms at the linking site and Au adatoms in the hGDY are also reported.

## Density of states of the pristine hGDY and aGNR

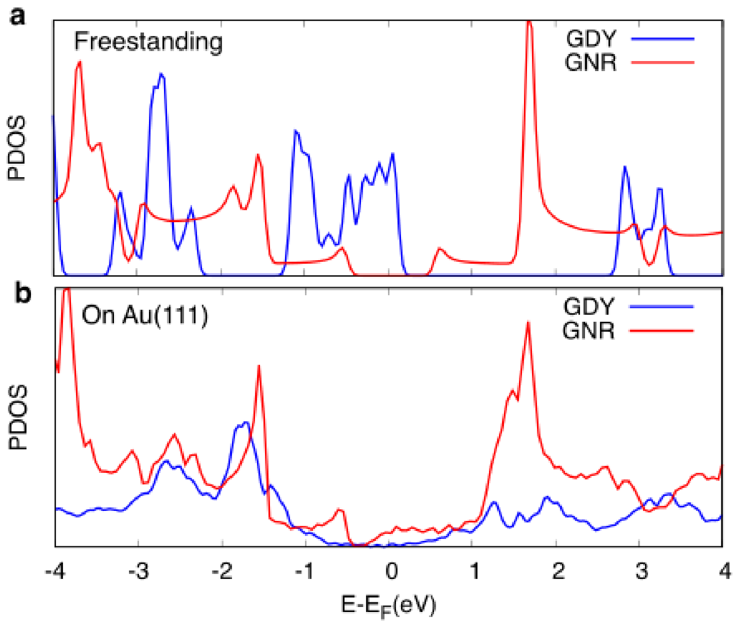


**Figure S11**: PDOS of the freestanding (a) and Au(111) supported (b) hGDY and aGNR

# Additional eigenchannels below the Fermi level at -0.23 eV

In Figure S12, three additional eigenchannels with transmission probability nearly equal to 1, calculated near the Fermi level (E=-0.2 eV), are reported (the first eigenchannel is displayed in the main text). They are all localized on the hGDY.

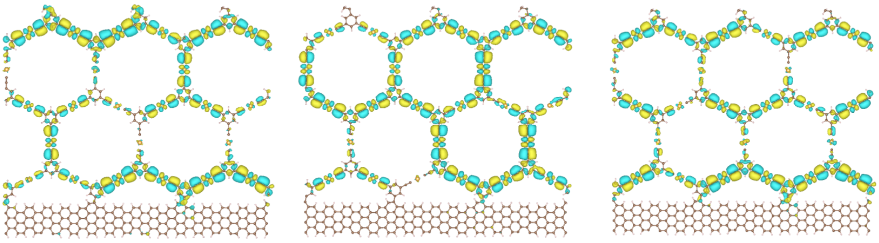

**Figure S12**: Eigenchannels $t_2$, $t_3$ and $t_4$ for E=-0.2 eV.

## PDOS and transmission of the “1H” freestanding configuration

In the freestanding case, the “1H” configuration is slightly less stable than “2H”, unlike the supported case in which 1H is stabilized. For the sake of completeness, in Figure S13 the PDOS and transmission of the “1H” freestanding configuration are reported, for which the same conclusions reported in the main manuscript hold. In particular the separation of the electronic states of the two subsystems, with the presence of a gap just above the Fermi level, leads to eigenchannels that, depending on the energy, show different spatial distribution of the current in the heterojunction.

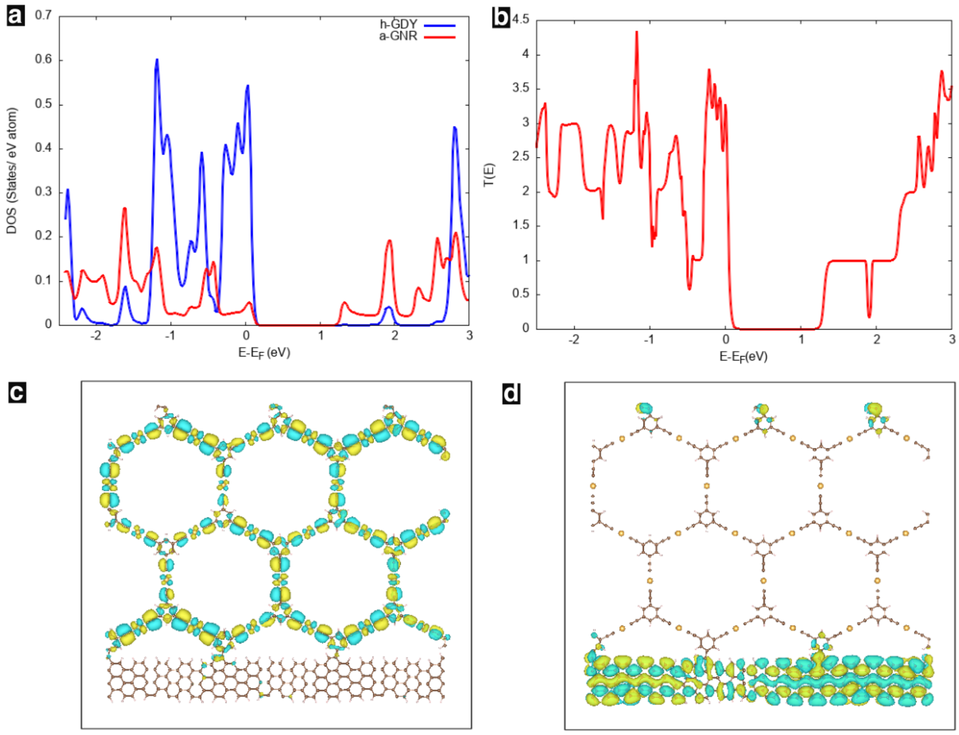


**Figure S13**: a) PDOS on a-GNR (red) and h-GDY (blue) carbon atoms. b) Transmission of the freestanding “1H” heterojunction. c) Eigenchannel at E=-0.2 eV. d) Eigenchannel at E=1 eV

## hGDY nucleation from aGNRs

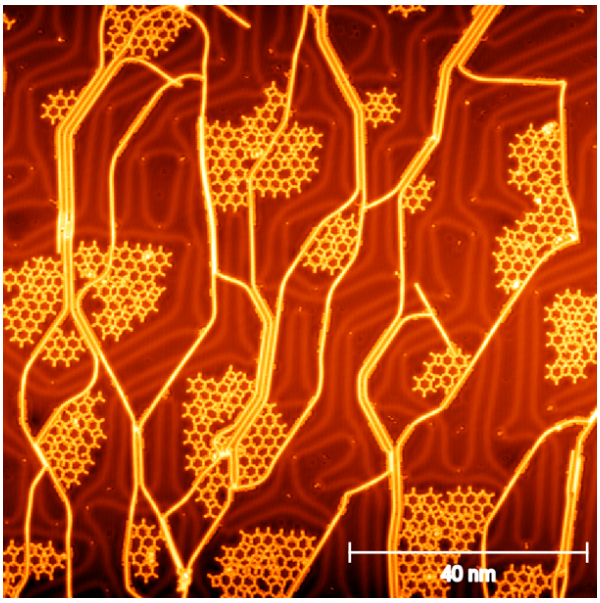


**Figure S14**: Large-scale LT-STM image of the low coverage as-deposited hGDY-aGNR heterostructure. STM setpoint: 500mV/50pA.
